# Supplementary material for: Demonstration of Einstein-Podolsky-Rosen Steering Using Hybrid Continuous- and Discrete-Variable Entanglement of Light
Source: arXiv:1811.00036 ancillary file (2018-10-31)
Supplement: Supplementary file 1 [file SM_HybridSteering_arxiv.pdf]

# Demonstration of Einstein-Podolsky-Rosen Steering Using Hybrid Continuous- and Discrete-Variable Entanglement of Light - Supplemental Material -

A. Cavaillès,<sup>1</sup> H. Le Jeannic<sup>†,1</sup> J. Raskop,<sup>1</sup> G. Guccione,<sup>1</sup> D. Markham,<sup>2</sup>  
E. Diamanti,<sup>2</sup> M. D. Shaw,<sup>3</sup> V. B. Verma,<sup>4</sup> S. W. Nam,<sup>4</sup> and J. Laurat<sup>1,\*</sup>

<sup>1</sup>*Laboratoire Kastler Brossel, Sorbonne Université, CNRS,*

*ENS-Université PSL, Collège de France, 4 Place Jussieu, 75005 Paris, France*

<sup>2</sup>*Laboratoire d'Informatique de Paris 6, Sorbonne Université, CNRS, 4 Place Jussieu, 75005 Paris, France*

<sup>3</sup>*Jet Propulsion Laboratory, California Institute of Technology,*

*4800 Oak Grove Drive, Pasadena, California 91109, USA*

<sup>4</sup>*National Institute of Standards and Technology, 325 Broadway, Boulder, CO 80305, USA*

## S1- CONDITIONAL ASSEMBLAGE

The measurements  $\theta = n * \pi/6$ , with  $n \in [0, 5]$  made by Alice –quadrature measurements at the corresponding local oscillator phase  $\theta$ – and the result  $a = \pm$  obtained with probability  $p(a|\theta)$ , lead to a set of conditional states  $\rho_{a|\theta}$ . The result of measurements  $\theta$  is signed binned and the corresponding measurement operators  $\hat{M}_\theta^\pm$  can be written as:

$$\begin{aligned}\hat{M}_\theta^+ &= \int_0^{+\infty} |qe^{i\theta}\rangle \langle qe^{-i\theta}| dq \\ \hat{M}_\theta^- &= \int_{-\infty}^0 |qe^{i\theta}\rangle \langle qe^{-i\theta}| dq\end{aligned}\quad (1)$$

Applying the operators on the DV mode of our hybrid state  $|\Psi\rangle_{AB} = \sqrt{R}|0\rangle_A|\text{CSS}_-\rangle_B - \sqrt{1-R}|1\rangle_A|\text{CSS}_+\rangle_B$ , we obtain

$$\begin{aligned}\rho_{a|\theta} &= \frac{\text{Tr}_A(\hat{M}_\theta^a |\Psi\rangle \langle \Psi|_{AB})}{\text{Tr}(\hat{M}_\theta^a |\Psi\rangle \langle \Psi|_{AB})} \\ \rho_{a|\theta} &\propto a R \int_0^{a\infty} dq |\langle 0|q\rangle|^2 |\text{CSS}_-\rangle \langle \text{CSS}_-| \\ &\quad + a (1-R) \int_0^{a\infty} dq |\langle 1|q\rangle|^2 |\text{CSS}_+\rangle \langle \text{CSS}_+| \\ &\quad + a \sqrt{R(1-R)} (e^{i\theta} \int_0^{a\infty} dq \langle 1|q\rangle \langle q|0\rangle |\text{CSS}_-\rangle \langle \text{CSS}_+| \\ &\quad + e^{-i\theta} \int_0^{a\infty} dq \langle 0|q\rangle \langle q|1\rangle |\text{CSS}_+\rangle \langle \text{CSS}_-|).\end{aligned}\quad (2)$$

Multiplying by  $p(a|\theta)$  the normalized  $\rho_{a|\theta}$ , we obtain the assemblage:

$$\begin{aligned}\sigma_{a|\theta} &= p(a|\theta) \rho_{a|\theta} \\ &= p(a|\theta) (R |\text{CSS}_-\rangle \langle \text{CSS}_-| \\ &\quad + (1-R) |\text{CSS}_+\rangle \langle \text{CSS}_+| \\ &\quad + a e^{i\theta} \sqrt{2R(1-R)/\pi} |\text{CSS}_-\rangle \langle \text{CSS}_+| + \text{h.c.}).\end{aligned}\quad (3)$$

<sup>†</sup> Present address: Niels Bohr Institute, University of Copenhagen, Blegdamsvej 17, DK-2100 Copenhagen, Denmark.

## S2- PRINCIPLE OF THE ERROR BAR COMPUTATION

EPR steering is demonstrated in our experiment by applying operators on the result of quantum state estimation (QSE) algorithms that use the function of likelihood  $\mathcal{L}$ . From a set of positive operator valued measures POVM  $\{M_k\}$ , the likelihood function is defined as the probability of a given density matrix  $\rho$  to have led to the observed data:

$$\mathcal{L}(\rho) = \prod_k \text{Tr}(M_k \rho). \quad (5)$$

Typically, QSE is performed by finding the density matrix  $\rho^{\text{ML}}$  that maximizes  $\mathcal{L}$  through a Maximum-Likelihood (ML) optimization process. From this result any figure of merit  $f$  such as purity, negativity of the Wigner function, or in our case  $\mathcal{S}$ , can be obtained by computing the expectation value of the relevant observable for  $\rho^{\text{ML}}$ . To construct error bars,  $\rho^{\text{ML}}$  is not sufficient, we need to consider density matrices for which the likelihood function is close to maximum.

We use the method proposed in [1] to compute an operational parameter -called *quantum error bar*- from which one can derive robust operational statements for error estimation such as the construction of confidence regions. The first step is to transform the function of likelihood  $\mathcal{L}(\rho)$  into a distribution by multiplying it by a prior distribution  $\pi(\rho)d\rho$ . This prior distribution represents the knowledge we have of our state prior to the experiment. In the context of the steering test we consider, we chose a fully indifferent prior, i.e., we make no prior assumption on the states observed and postulate  $\pi(\rho)d\rho = \frac{1}{c}d\rho$ , with  $c$  a normalizing factor such that  $\int \frac{1}{c}\mathcal{L}(\rho)d\rho = 1$ . The knowledge of  $\frac{1}{c}\mathcal{L}(\rho)d\rho$  allows the computation of the statistics of any figure of merit  $f$  by reconstructing the reduced distribution  $\mu(f) = \int \frac{1}{c}\mathcal{L}(\rho)\delta(f(\rho) - f)d\rho$ . Using a Metropolis-Hastings (MH) algorithm, one can evaluate  $\mu(f)$  —without the knowledge of the normalisation constant  $c$ — and deduce from it the *quantum error bars* associated to the computation of  $f$ .

In our case, we aim to evaluate the error bars on the

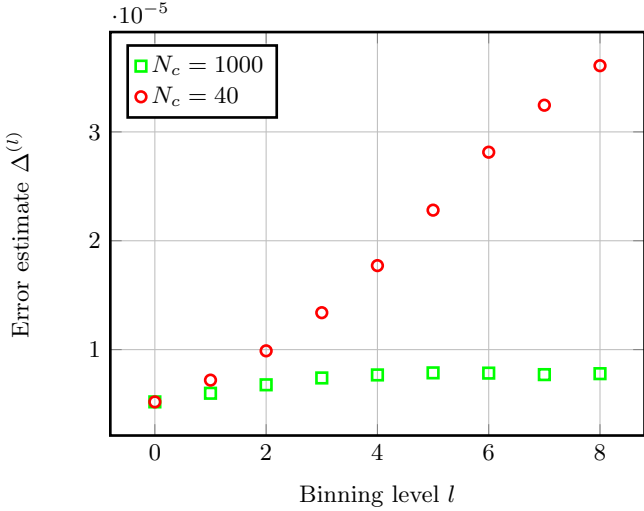

FIG. 1: Binning analysis of  $f_{a|\theta}(\rho)$  averaged over  $a$  and  $\theta$  for two data sets of size  $M = 10000$  with different sample rejection rates  $N_c$ . We can see that convergence is reached only for the sample build with  $N_c = 1000$  for a binning level  $l \geq 5$ . This data allows the computation of the integrated auto-correlation time of each data set  $A_{a|\theta}^{(0)}$  as the error bars on  $\mu(f_{a|\theta})$ .

measurement of  $\mathcal{S} = \text{Tr}(\sum F_{a|\theta} \sigma_{a|\theta})$ , meaning that we need to find for each  $\rho_{a|\theta}$  the statistics of the figure of merit  $f_{a|\theta}(\rho) = \text{Tr}(F_{a|\theta} \rho(a|\theta) \rho)$  and therefore compute each  $\mu(f_{a|\theta})$ . Note that the steering scenario may add constraints linking the various  $\mu(f_{a|\theta})$  (especially between  $\mu(f_{+|\theta})$  and  $\mu(f_{-|\theta})$  for every  $\theta$ ) but we computed each of them separately as this can only lead to an over-estimation of uncertainties. The resulting  $\mu(f_{a|\theta})$  functions are then combined to find  $\mu(\mathcal{S})$  from which we can determine the error bars on  $\mathcal{S}$ .

### S3- PARAMETERS USED AND DETAILS OF THE METROPOLIS-HASTINGS EXPLORATION

The computations were done in a Hilbert space of dimension 10 spanned by Fock states  $|0\rangle, |1\rangle, \dots, |9\rangle$  (In practice we see a convergence of results for spaces of dimensions greater than 7). The MH algorithm amounts to a random walk in state space biased by the likelihood function to obtain a set of density matrices  $\{\rho_i\}$ . At every step, a candidate density matrix  $\rho_c$  is chosen according to a jump distribution centered on  $\rho_i$ . The next density matrix  $\rho_{i+1}$  is then set either following  $\rho_{i+1} = \rho_c$  with probability  $\min(1, \mathcal{L}(\rho_c)/\mathcal{L}(\rho_i))$  or else following  $\rho_{i+1} = \rho_i$ . The values  $f_{a|\theta}(\rho_i)$  are recorded and after a great number of iterations will be distributed according to  $\mu(f_{a|\theta})$ .

We chose a gaussian jump distribution with a standard deviation set so that we would observe a jump close to 23% of the time, the ideal value to efficiently

explore the state space [2]. As the MH algorithm is an iterative process, correlations between samples have to be taken into account and in our case keeping only one out of  $N_c = 1000$  values of  $f_{a|\theta}(\rho_i)$  and accumulating  $M = 10000$  samples was enough to circumvent their effect. This was verified by computing the sample set's *integrated autocorrelation time*  $\tau_A$  [3]. This parameter indicates the distance between two uncorrelated samples in the data set and can be computed through a binning analysis. This process consists of creating, from the original data set  $A_{a|\theta}^{(0)} = \{f_{a|\theta}(\rho_i)\}_{i \leq M}$ , several binned series by averaging consecutive entries following:

$$A_{a|\theta}^{(l)} = \frac{1}{2} \{A_{a|\theta, 2i-1}^{(l-1)} + A_{a|\theta, 2i}^{(l-1)}\}_{i \leq M/2^l}. \quad (6)$$

For each of these  $A_{a|\theta}^{(l)}$  we can then compute the error estimate  $\Delta_{a|\theta}^{(l)} = \sqrt{\text{Var}(A_{a|\theta}^{(l)}) * 2^l / M}$ .

To show the effect of  $N_c$ , we compared two data sets of size  $M = 10000$  constructed independently with parameters  $N_c = 40$  and  $N_c = 1000$ . We denote as  $\Delta^{(l)}$  the average over  $\theta$  and  $a$  of  $\Delta_{a|\theta}^{(l)}$ . In Fig. 1 we show the evolution of  $\Delta^{(l)}$  with  $l$  for both sets. Only the second set sees convergence for  $l \geq 5$  which ensures the sampling to be adequate and allows us to compute  $\tau_A = \frac{1}{2} ((\frac{\Delta^{(\infty)}}{\Delta^{(0)}})^2 - 1) \approx 0.65$ . This means the sample neighbours are typically uncorrelated on average for all  $\theta$  and  $a$ .

The histogram  $\mathcal{H}(f_{a|\theta}, M)$  obtained from the data set  $A_{a|\theta}^{(0)}$  is therefore a valid evaluation of  $\mu(f_{a|\theta})$  up to a deviation that can be computed using  $\tau_{a|\theta}$ . Considering the histogram as the data set  $\{p_n, \mathcal{I}_n\}$ , with  $p_n$  the normalized number of values  $f_{a|\theta}$  comprised in the interval  $\mathcal{I}_n$ , the error on each  $p_n$  is estimated at

$$\delta_{a|\theta}(n) = \sqrt{\frac{p_n - p_n^2}{M/(1 + 2\tau_{a|\theta}) - 1}}.$$

By summing random members of all  $A_{a|\theta}^{(0)}$  data sets  $N$  times we then obtained  $A_{\mathcal{S}}$ , our final set of  $\mathcal{S}$  values. To ensure an accurate sampling of our data, we chose  $N = 5 * 10^8$  and were then able to compute the corresponding histogram  $\mathcal{H}(\mathcal{S}, N)$ . As  $\mathcal{S}(\rho) = \sum f_{a|\theta}(\rho)$ , the error on each point of  $\mathcal{H}(\mathcal{S}, N)$  was evaluated to be

$$\delta(n) = \sqrt{\frac{1}{12^2} \sum_{a, \theta} \delta_{a|\theta}(n)^2}.$$

Using this information,  $\mathcal{H}(\mathcal{S}, N)$  is shown in green in Fig. 2 along with the sets  $\{p_n \pm \delta(n)/2, \mathcal{I}_n\}$  that bound the area containing  $\mu(\mathcal{S})$  with a confidence of one standard deviation ( $1\sigma$ ). As a comparison, the same evaluation was done using  $N_c = 40$  and is shown in red. The results for both independent sets are compatible and show

the relevance of moving to a higher sample rejection rate for a more precise evaluation of our error bars. A numerical fitting of  $\mu(\mathcal{S})$  shows good agreement with a gaussian distribution so no deskewing procedure [1] was found necessary. As a result the standard deviation of our data set  $A_{\mathcal{S}}$  is a direct evaluation of the errors associated to our MaxLik reconstruction. The final fitting of our data is a gaussian of mean  $x_0 = -0.00992 \pm 0.00010$  and standard deviation  $\sigma = 0.00181 \pm 0.00004$ , which gives a separation to the local bound of  $-5.48\sigma \pm 0.18\sigma$ .

Additional iterations of the MH algorithm would render the sample correlation's bias negligible compared to the sample size but would necessitate significant computational time.

Other bias sources have been considered as well. The first  $N_{\theta} = 1250$  samples have to be rejected to record data only in a region of non-negligible likelihood value. This is referred as having reached thermalization [2]. Many independent runs of the MH algorithm have been launched to verify similar  $\mathcal{S}$  values are obtained after thermalization has occurred when starting from different points of state space. This gives us confidence in the uniformity of the explored space and justifies the use of a single long run to compute our final result.

#### S4- COMPARISON WITH THE BOOTSTRAPPING METHOD

As a point of comparison, we performed the generally-used bootstrap analysis of our data. The bootstrap method we use is parametrized by  $\rho^{\text{ML}}$ , the density matrix found using a Maximum-Likelihood algorithm on our

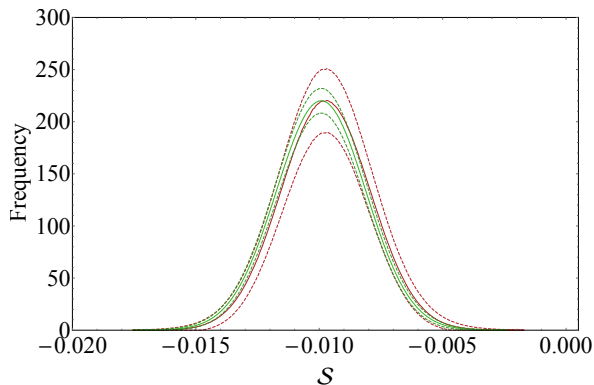

FIG. 2: Histogram of the steering parameter values for  $N = 5 \times 10^8$  points out of two data sets of size  $M = 10^4$  computed with parameters  $N_c = 40$  in red and  $N_c = 1000$  in green. The area delimited by dashed lines encompass possible histograms at less than one standard deviation from the average. The green histogram is the final evaluation of the error bars associated to the steering inequality violation. We observe a distance to the local bound of more than 5 standard deviations.

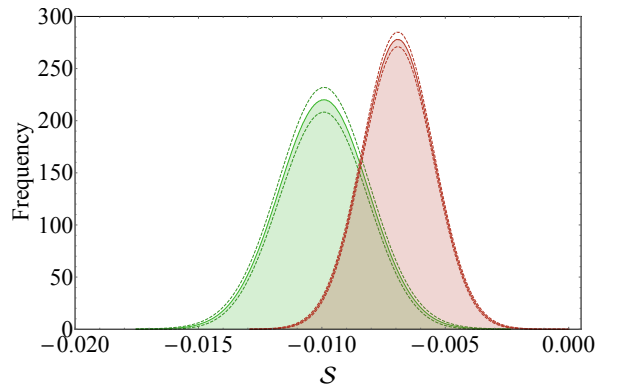

FIG. 3: Histogram of the steering parameter values for  $5 \cdot 10^8$  points out of a set of  $12 \cdot 10^4$  density matrices using the bootstrap method (in red) and using the quantum error bar approach (in green).

quadrature data, and the total number of measurements we made which amounts to  $N_{mes} = 6 \times 10^4$  on average over  $a$  and  $\theta$ . The process is repeated a number of times. Each time  $N_{mes}$  quadrature measurements are simulated following the probability distribution determined by  $\rho^{\text{ML}}$ . Once obtained, the simulated results are run through a ML algorithm to obtain a set of reconstructed density matrices  $\{\rho_{a|\theta}^{(p)}\}_{p \leq M}$ . Applying operators  $F_{a|\theta}$  to the density matrices ensembles we can reconstruct similarly as before an histogram  $\mathcal{H}^{BS}(\mathcal{S}, N)$  from which we obtain the error estimation given by the bootstrap method.

In Fig. 3 we show the bootstrap technique results in red, the estimated distance to the local bound is  $4.8\sigma$ . We therefore have a slight difference between the two methods, as expected, even though the steerability of our assemblage is verified in both cases.

\* Electronic address: julien.laurat@sorbonne-universite.fr

- [1] P. Faist and R. Renner, Practical and Reliable Error Bars in Quantum Tomography, *Phys. Rev. Lett.* **117**, 010404 (2016).
- [2] G. O. Roberts and J. S. Rosenthal, Optimal Scaling for Various Metropolis-Hastings Algorithms, *Stat. Sci.* **16**, 351 (2001).
- [3] V. Ambegaokar and M. Troyer, Estimating errors reliably in Monte Carlo simulations of the Ehrenfest model, *Am. J. Phys.* **78**, 150 (2010).
